# Supplementary material for: Rudraksh: A compact and lightweight post-quantum key-encapsulation mechanism
Source: arXiv:2501.13799 source file (2025-01-23)
Supplement: Supplementary file 1 [file appendix.tex]

\subsection{Description on MLWE-based Public-key \\Encryption}~\label{app:pke}

Here we explain the MLWE-based PKE presented in Fig.~\ref{fig:kyberpke} in Sec.~\ref{lwe-pke}.
The public matrix $\pmb{A}$ is drawn from $R_q^{n(l\times l)}$ uniformly randomly, and this implies $\pmb{\hat{A}}=\mathtt{NTT}(\pmb{A})$ is also uniformly random in $R_q^{n(l\times l)}$. So, we sample $\pmb{\hat{A}}$ from $R_q^{n(l\times l)}$ in order to avoid calculating $\mathtt{NTT}(\pmb{A})$. $\pmb{\hat{A}}$ is generated using a pseudorandom function (\texttt{PRF}) and random input $seed_{\pmb{A}}$. $seed_{\pmb{A}}$ is send as the part of public-key $pk$ instead of $\pmb{\hat{A}}$ by the \texttt{PKE.KeyGen} algorithm to reduce the size of the $pk$. The $l$-length vector of polynomials secret $\pmb{s}$ and noise $\pmb{e}$ are sampled using narrow CBD and $seed_{\pmb{se}}$ in the \texttt{PKE.KeyGen} algorithm. The other part of the public-key $pk$ is the LWE instance $\pmb{\hat{b}} = \pmb{\hat{A}}\circ \pmb{\hat{s}} + \pmb{\hat{e}}$. In \texttt{PKE.KeyGen} algorithm, the $l$-length secret vector of polynomials $\pmb{s}$ and the $l$-length noise vector of polynomials $\pmb{e}$ are sampled using narrow CBD $\beta_\mu$ and random input $seed_{\pmb{se}}$. The other part of the public-key $pk$ is the LWE instance $\pmb{\hat{b}} = \pmb{\hat{A}}\circ \pmb{\hat{s}} + \pmb{\hat{e}}$. 

The ciphertext $c$ generated from the \texttt{PKE.Enc} algorithm has two parts $(\pmb{u},v)$, where $\pmb{u}$ is the key possessed part and $v$ is the ciphertext contained part. $\pmb{u}$ is generated from the application of $\mathtt{Compress}:R_q^n\longrightarrow R_p^n$ operation on $\pmb{b'}$. $\pmb{b'} = \mathtt{INTT}(\pmb{\hat{A}}\circ \mathtt{NTT}(\pmb{s'}))+\pmb{e'} = \pmb{A}\cdot\pmb{s'}+\pmb{e'}$ is a MLWE instance of \texttt{PKE.Enc} similar to $\pmb{\hat{b}}$ of \texttt{PKE.KeyGen}. The only difference is that $\pmb{\hat{b}}$ is in the NTT domain, whereas $\pmb{b'}$ is the normal domain. The $\mathtt{Compresss}$ operation on $\pmb{b'}$ is performed and generated $\pmb{u}$ to reduce the size of the ciphertext. The other part of the ciphertext $v$ contains the encoding of the message $m$. $v=\pmb{b}\cdot \pmb{s'}+e''+\mathtt{Encode}(m)$, where $b=\mathtt{INTT(\pmb{\hat{b}})}$ and $\mathtt{Encode}: R_{2^B}^n\longrightarrow R_q^n$ such that $\mathtt{Encode}(m) = \lfloor \frac{q}{2^B}\rceil m$. Here, each coefficient of $v$ stores $B$ message bits. 

\texttt{PKE.Dec} decompresses the ciphertext $c=(\pmb{u},\ v)$ to $(\pmb{u'}, v')$ and then computes $m'' = v' - \pmb{u'}\cdot s$. $m''=\mathtt{m}+\pmb{e}\cdot \pmb{s'}-\pmb{e'}\cdot \pmb{s}+e''$ is a noisy version of the encrypted message. $\pmb{e}\cdot \pmb{s'}-\pmb{e'}\cdot \pmb{s}+e''$ is called decryption noise. Then $\mathtt{Decode}: R_q^n\longrightarrow R_{2^B}^n$ such that $\mathtt{Decode}(m'')=\frac{2^Bm''+\lfloor q/2\rceil}{q}\&(2^B-1)$ is performed on $m''$ to remove decryption noise from the encrypted message.

\subsection{Description on MLWE-based \\Key Encapsulation Mechanism}~\label{app:kem}

\texttt{KEM.KeyGen} is similar to \texttt{PKE.KeyGen} which generates public-key $\overline{pk}$ and secret-key $\overline{sk}$. Public-key of \texttt{KEM.KeyGen}, $\overline{pk}$ is the same as the public-key $pk$ of \texttt{PKE.KeyGen}. Secret-key of \texttt{KEM.KeyGen}, $\overline{sk}$ contains the secret-key $sk$ of \texttt{PKE.KeyGen} together with the hash of $pk$ ($\mathcal{H}$) and a random $\text{len}_K$ bits number $z$. This random number $z$ is used in the case of decryption failure. \texttt{KEM.Encaps} takes $\overline{pk}$ as input and generates $\text{len}_K$ bits message $m$ and perform hash $\mathcal{G}$ on $(\mathcal{H}(pk),\ m)$ and generates the shared key $K$. Then it uses \texttt{PKE.Enc} to generate the ciphertext $c$. Here, the derivation of the shared key $K$ does not include the hash of the ciphertext $c$ like ML-KEM~[cite{XX}]. \texttt{KEM.Decaps} algorithm first decrypts the ciphertext $c$ using \texttt{PKE.Dec} algorithm and then compute the shared key $K'$ using the decrypted message $m'$ and perform hash $\mathcal{G}$ on $(\mathcal{H}(pk),\ m')$. After that, a re-encryption process is invoked with the message $m'$ and using \texttt{PKE.Enc}. Then, a ciphertext checking is performed. If the re-encrypted ciphertext is the same as the public ciphertext, then a decapsulation success is occurred. \texttt{KEM.Decaps} algorithm returns the shared key $K'(=K)$. Otherwise, a decapsulation failure will occur, and then the decapsulation algorithm returns a random number $K''$ using hash $\mathcal{H}$ on the public ciphertext $c$, and the random key $z$. 

\subsection{NTT and INTT algorithm}~\label{app:ntt-intt}
\begin{algorithm}[!ht]
\caption{NTT algorithm~\cite{patrick_longa_ntt} }
\label{algo:ntt}
\Input{$x$, where $x$ is a polynomial in $R_q^n$}
\Output{$\hat{x} = \mathtt{NTT}(x)$}
% \BlankLine
% \BlankLine
$m = 1$\\
\For{$\mathtt{layer=}$ $\log_2n-1$ \text{down to} $1$ \text{by} $1$}
{
    $d = 2^{\mathtt{layer}}$\\
    \For{\texttt{len=} $0$ \text{to} $n-1$  \text{by} $d$}
    {
        $\mathtt{zeta} = \zeta^{\mathtt{bitreverse}(m)}$ $\vartriangleright${pre-computed}\\
        \For{$j = len$ \texttt{to} $\mathtt{len}+d$ by $1$}
        {
            $t = \mathtt{zeta}*x[j+d] \bmod{q}$\\
            $x[j+d] = (x[j] - t) \bmod{q}$\\
            $x[j] = (x[j] + t) \bmod{q}$\\ 
        }                
        $m = m+1$\\
    }
}
% $\hat{x} = {x}$\\
\algorithmicreturn{ $\hat{x}=x$}
\end{algorithm}

\begin{algorithm}[!ht]
\caption{INTT algorithm~\cite{intt_by_2} }
\label{algo:intt}
\Input{$\hat{x}$, where $\hat{x} = \mathtt{NTT}(x) \in \mathbb{Z}_q^n$ is in point value domain}
\Output{${x} = \mathtt{INTT}(\hat{x})$}
% \BlankLine
% \BlankLine
$m = n-1$\\
\For{$\mathtt{layer=}$ $1$ \text{to} $\log_2n-1$  \text{by} $1$}
{
    $d = 2^{\mathtt{layer}}$\\
    \For{\texttt{len=} $0$ \text{to} $n-1$ \text{by} $d$}
    {
        $\mathtt{zeta} = \zeta^{\mathtt{bitreverse}(m)}$     $\vartriangleright${pre-computed}\\
        \For{$j = len$ \text{to} $\mathtt{len}+d$ \text{by} $1$}
        {
            $t = \hat{x}[j]$\\
            $t1 = (x[j+d] + t) \bmod{q}$\\
            $\hat{x}[j] = (t1\gg1)+(\frac{q+1}{2}*(t1\&1))$ \hfill $\rhd$ $\mathtt{div\_by\_2}()$\\
            $t2 = (\mathtt{zeta}*(\hat{x}[j+d] - t)) \bmod{q}$\\ 
            $\hat{x}[j+d] = (t2\gg1)+(\frac{q+1}{2}*(t2\&1))$ \hfill $\rhd$ $\mathtt{div\_by\_2}()$\\
        }                
        $m = m-1$\\
    }
}
% ${x} = \hat{x}$\\
\algorithmicreturn{ ${x}=\hat{x}$}
\end{algorithm}

\subsection{Description of ASCON-XOF}~\label{app:ascon}
ASCON-XOF function~\cite{ASCON}, presented in Fig.~\ref{fig:ascon}, has three steps: a) initialization, b) absorb, and c)squeeze. The initial state register is pre-computed from $IV$ in our design to save latency. Then padding is performed on the input steam to accommodate the inputs whose bit sizes are not multiples of $64$. The second step is to absorb the input stream in the block of $64$ bits. 
During absorb, $64$ bits input block is XORed with the first $64$ bits of the state register followed by $p^{12}$. The third step is to squeeze the output bits. In ASCON, $64$ bits of outputs are generated after a $12$ rounds of permutation $p^{12}$. This process continues until the required length of output is extracted. ASCON permutation $p^{12}$ is the primary building block used during all three steps: (i) addition of constant round, (ii) substitution layer, and (iii) linear diffusion layer. $320$-bit state register of ASCON is divided into five $64$ bits registers. In the constant addition round, a single-byte constant is XORed with the third $64$ bits register between the five registers. In the substitution layer, 64 parallel $5$-bit S-box is applied on the five registers (in bit-sliced style). The diffusion occurs within each $64$ bits register in the linear diffusion layer using circular shift and bit-wise XOR operations.
